# Supplementary material for: Multireference configuration interaction study of the predissociation of C$_{2}$ via its $F\,^1\Pi_u$ state
Source: arXiv:2206.03540 source file (2022-06-07)
Supplement: Supplementary file 1 [file C2_calc_SI.pdf]

# Multireference configuration interaction study of the predissociation of $C_2$ via its $F\,^1\Pi_u$ state

Zhongxing Xu (徐重行), William M. Jackson,
Cheuk-Yiu Ng, Lee-Ping Wang, and Kyle N. Crabtree
*Department of Chemistry, University of California – Davis*

S. R. Federman
*Department of Physics and Astronomy, University of Toledo*
(*kncrabtree@ucdavis.edu)

TABLE I. List of machine-readable tables

| Table | description |
|---|---|
| Table S1 | MRCI+Q/aug-cc-pV5Z-2s2p PECs for all electronic states of $C_2$ |
| Table S2 | TDMs from the ground $X$ state to other electronic states of $C_2$ |
| Table S3 | TDMs from the $F\,^1\Pi_u$ state to other electronic states of $C_2$ |
| Table S4 | Photodissociation cross section of $C_2$ via the $F\,^1\Pi_u - X\,^1\Sigma_g^+$ transition in the range of 72000-80000 $\mathrm{cm}^{-1}$ range |

As shown in Table I, the PECs of all 56 states obtained from the MRCI+Q calculations described in the main text are given in Table S1. The TDMs between excited electronic states and the ground $X\,^1\Sigma_g^+$ state are reported in Table S2. The TDMs between the $F\,^1\Pi_u$ state and lower-energy states are presented in Table S3. The values in Tables S2 and S3 are not phase corrected. The rotationless photodissociation cross sections via the $F\,^1\Pi_u - X\,^1\Sigma_g^+$ transition are given in Table S4. While Figure 13 in the main text shows a wider frequency range, only data in 72000-80000 $\mathrm{cm}^{-1}$ range, which covers the $F - X$ (0-0) and (1-0) bands, are in Table S4.
